# Supplementary material for: Leveraging Domain Features for Detecting Adversarial Attacks Against Deep Speech Recognition in Noise
Source: arXiv:2211.01621 source file (2022-11-03)
Supplement: Supplementary file 1 [file appendix.tex]

\appendix

\section{Appendix}

Optionally include extra information (complete proofs, additional experiments and plots) in the appendix.
This section will often be part of the supplemental material.
